# Supplementary material for: Exact electronic states with shallow quantum circuits through global optimisation
Source: arXiv:2207.00085 ancillary file (2022-06-30)
Supplement: Supplementary file 1 [file supplementary_material.pdf]

# Exact electronic states with shallow quantum circuits through global optimisation: Supplementary Material

Hugh G. A. Burton,[1, a] Daniel Marti-Dafcik,[1] David P. Tew,[1] and David J. Wales[2]
[1] Physical and Theoretical Chemistry Laboratory, University of Oxford, South Parks Road, Oxford, OX1 3QZ, U.K.
[2] Yusuf Hamied Department of Chemistry, University of Cambridge, Lensfield Road, Cambridge, CB2 1EW, U.K.

(Dated: 30 June 2022)

**Contents**

**S1. Universality of one-body and paired two-body operator pool** 2

**S2. Qubit operators and quantum circuit implementation** 3
S2.1. General operators 3
S2.2. Operators in s-UPS ansatz 4
S2.3. Circuit costs 4

**S3. Summary of the DISCO-VQE algorithm** 4
S3.1. Continuous optimisation using basin-hopping 4
S3.2. Performing discrete steps 5
S3.3. Taking uphill discrete steps 7
S3.4. Summary of hyperparameters 9
S3.5. Computational implementation 9

**S4. Linear and tetrahedral $H_4$ (STO-3G)** 10
S4.1. Computational Details 10
S4.2. Binding curve using a fixed *ansatz* 10
S4.3. Comparison of DISCO-VQE and ADAPT-VQE binding curves 10

**S5. Linear $H_6$ binding curve (STO-3G)** 11
S5.1. Computational Details 11

**S6. Symmetric $H_2O$ binding curve (STO-3G)** 11
S6.1. Computational Details 11

**S7. $N_2$ binding curve (STO-3G)** 11
S7.1. Computational Details 11
S7.2. Comparison of binding curve accuracy 12

**S8. Two-dimensional Hubbard lattice** 12

**S9. References and Notes** 12

[a] Electronic mail: hgaburton@gmail.com

## S1. Universality of one-body and paired two-body operator pool

In the main text, we show that an arbitrary wave function can be represented as a unitary product state using only one- and paired two-body fermionic operators. The universality of this *ansatz* arises as an extension to the proof presented for Disentangled Unitary Coupled Cluster in Ref. 9. In that work, it was shown that any exact state can be built as a unitary product of generalised one-body and two-body operators. This is achieved by decomposing higher-body operators, which appear in the disentangled exact wave function, into nested commutators of one- and two-body operators, which can then be expanded as a product of individual unitary operators.[9] Here, we show that this derivation can be extended to restrict the operator pool to only paired two-body operators. In particular, we show that unpaired two-body operators can be decomposed into commutators that include only one-body and paired two-body operators as

$$\left[\left[\hat{\kappa}_{\bar{r}}^{\bar{s}}, \hat{\kappa}_{p\bar{p}}^{r\bar{r}}\right], \hat{\kappa}_{\bar{q}}^{\bar{p}}\right] = \hat{\kappa}_{p\bar{q}}^{r\bar{s}}, \tag{S1a}$$

$$\left[\hat{\kappa}_{p\bar{q}}^{r\bar{s}}, \hat{\kappa}_{s\bar{s}}^{q\bar{q}}\right] = \hat{\kappa}_{ps}^{rq}(\hat{n}_{\bar{s}} - \hat{n}_{\bar{q}}). \tag{S1b}$$

Goldstone diagrams[45] for these commutator combinations are illustrated in Fig. S1. The additional factor $(\hat{n}_{\bar{s}} - \hat{n}_{\bar{q}})$ introduces number operators (e.g. $\hat{n}_{\bar{q}} = \hat{a}_{\bar{q}}^{\dagger}\hat{a}_{\bar{q}}$) that will create a stronger dependence on the ordering of unitary operators. However, since these commute with all (de)excitation operators, the commutator expansions for higher-order operators are unaffected and can be derived using the process described in Ref. 9.

To prove the commutator expansions in Eqs. (S1a) and (S1b), we exploit the general representation of fermionic excitation operators $\hat{E}_p^q = \hat{a}_q^{\dagger}\hat{a}_p$[7] and define $p \neq q \neq r \neq s$. The derivation for the commutator expansion in Eq. (S1a) starts with

$$\begin{aligned}
\left[\hat{\kappa}_{\bar{r}}^{\bar{s}}, \hat{\kappa}_{p\bar{p}}^{r\bar{r}}\right] &= \left(\hat{E}_{\bar{r}}^{\bar{s}} - \hat{E}_{\bar{s}}^{\bar{r}}\right)\left(\hat{E}_p^r\hat{E}_{\bar{p}}^{\bar{r}} - \hat{E}_r^p\hat{E}_{\bar{r}}^{\bar{p}}\right) - \left(\hat{E}_p^r\hat{E}_{\bar{p}}^{\bar{r}} - \hat{E}_r^p\hat{E}_{\bar{r}}^{\bar{p}}\right)\left(\hat{E}_{\bar{r}}^{\bar{s}} - \hat{E}_{\bar{s}}^{\bar{r}}\right) \\
&= \hat{E}_p^r\left[\hat{E}_{\bar{r}}^{\bar{s}}, \hat{E}_{\bar{p}}^{\bar{r}}\right] + \hat{E}_r^p\left[\hat{E}_{\bar{s}}^{\bar{r}}, \hat{E}_{\bar{r}}^{\bar{p}}\right] \\
&= \hat{E}_p^r\hat{E}_{\bar{p}}^{\bar{s}} - \hat{E}_r^p\hat{E}_{\bar{s}}^{\bar{p}} \\
&= \hat{\kappa}_{p\bar{p}}^{r\bar{s}},
\end{aligned} \tag{S2}$$

where we have exploited the general identities[10] $\left[\hat{E}_p^q, \hat{E}_r^s\right] = \hat{E}_r^q\,\delta_{ps} - \hat{E}_p^s\,\delta_{rq}$ and $\hat{E}_p^r\hat{E}_q^r = \hat{E}_r^p\hat{E}_r^q = 0$. The full commutator

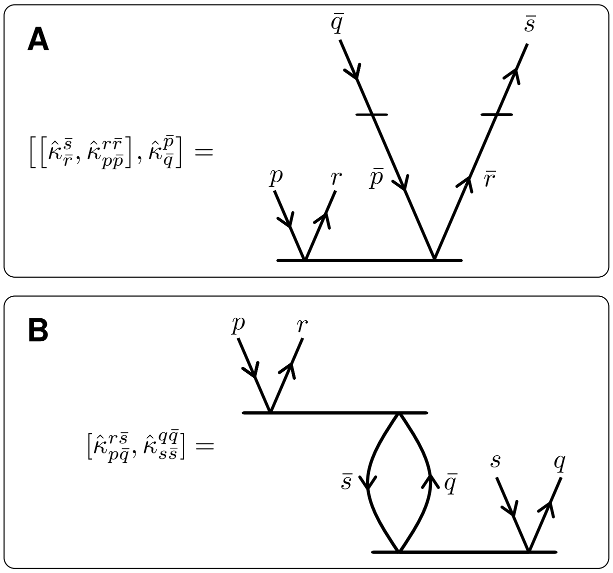


FIG. S1: Goldstone diagrams (**A**) and (**B**) represent the commutators in Eqs. (S1a) and (S1b), respectively.

expansion then follows by taking

$$\begin{aligned}[\hat{\kappa}^{r\bar{s}}_{p\bar{p}}, \hat{\kappa}^{\bar{p}}_{\bar{q}}] &= \left(\hat{E}^r_p \hat{E}^{\bar{s}}_{\bar{p}} - \hat{E}^p_r E^{\bar{p}}_{\bar{s}}\right)\left(\hat{E}^{\bar{p}}_{\bar{q}} - \hat{E}^{\bar{q}}_{\bar{p}}\right) - \left(\hat{E}^{\bar{p}}_{\bar{q}} - \hat{E}^{\bar{q}}_{\bar{p}}\right)\left(\hat{E}^r_p E^{\bar{s}}_{\bar{p}} - \hat{E}^p_r E^{\bar{p}}_{\bar{s}}\right) \\ &= \hat{E}^r_p \left[\hat{E}^{\bar{s}}_{\bar{p}}, \hat{E}^{\bar{p}}_{\bar{q}}\right] + \hat{E}^p_r \left[\hat{E}^{\bar{p}}_{\bar{s}}, \hat{E}^{\bar{q}}_{\bar{p}}\right] \\ &= \hat{E}^r_p \hat{E}^{\bar{s}}_{\bar{q}} - \hat{E}^p_r \hat{E}^{\bar{q}}_{\bar{s}} \\ &= \hat{\kappa}^{r\bar{s}}_{p\bar{q}}.\end{aligned} \tag{S3}$$

Continuing this approach allows Eq. (S1b) to be derived using the commutator expansion

$$\begin{aligned}[\hat{\kappa}^{r\bar{s}}_{p\bar{q}}, \hat{\kappa}^{q\bar{q}}_{s\bar{s}}] &= \left(\hat{E}^r_p \hat{E}^{\bar{s}}_{\bar{q}} - \hat{E}^p_r \hat{E}^{\bar{q}}_{\bar{s}}\right)\left(\hat{E}^q_s \hat{E}^{\bar{q}}_{\bar{s}} - \hat{E}^s_q \hat{E}^{\bar{s}}_{\bar{q}}\right) - \left(\hat{E}^q_s \hat{E}^{\bar{q}}_{\bar{s}} - \hat{E}^s_q \hat{E}^{\bar{s}}_{\bar{q}}\right)\left(\hat{E}^r_p \hat{E}^{\bar{s}}_{\bar{q}} - \hat{E}^p_r \hat{E}^{\bar{q}}_{\bar{s}}\right) \\ &= \left(\hat{E}^r_p \hat{E}^q_s - \hat{E}^p_r \hat{E}^s_q\right)[E^{\bar{s}}_{\bar{q}}, E^{\bar{q}}_{\bar{s}}] \\ &= \left(\hat{E}^r_p \hat{E}^q_s - \hat{E}^p_r \hat{E}^s_q\right)\left(\hat{E}^{\bar{q}}_{\bar{q}} - \hat{E}^{\bar{s}}_{\bar{s}}\right) \\ &= \hat{\kappa}^{rq}_{ps}(\hat{n}_{\bar{s}} - \hat{n}_{\bar{q}}).\end{aligned} \tag{S4}$$

On the last line, we have identified $\hat{E}^{\bar{q}}_{\bar{q}} = \hat{a}^\dagger_{\bar{q}} \hat{a}_{\bar{q}} = \hat{n}_{\bar{q}}$ as the number operator for spin-orbital $\bar{q}$. Through these expansions, we can expand any $n$-body fermionic operator as a series of nested commutators involving only one-body or paired two-body operators. Therefore, the unitary product states built with these operators are universal.

## S2. Qubit operators and quantum circuit implementation

### S2.1 General operators

General fermionic one-body and two-body operators are given by:

$$\hat{\kappa}^q_p = (\hat{a}^\dagger_q \hat{a}_p - \hat{a}^\dagger_p \hat{a}_q), \tag{S5a}$$

$$\hat{\kappa}^{rs}_{pq} = (\hat{a}^\dagger_r \hat{a}^\dagger_s \hat{a}_q \hat{a}_p - \hat{a}^\dagger_p \hat{a}^\dagger_q \hat{a}_s \hat{a}_r), \tag{S5b}$$

where the operators $\hat{a}^\dagger_p$ and $\hat{a}_p$ are creation and annihilation operators for spin-orbital $p$, respectively, and satisfy fermionic anticommutation relations $[\hat{a}_p, \hat{a}^\dagger_q]_+ = \delta_{pq}$, and $[\hat{a}_p, \hat{a}_q]_+ = [\hat{a}^\dagger_p, \hat{a}^\dagger_q]_+ = 0$. These fermionic operators can be mapped to qubit operators using the Jordan-Wigner transformation[3,20]

$$\hat{a}_p = \frac{1}{2}(X_p + \mathrm{i}\, Y_p) \prod_{k=1}^{p-1} Z_k \tag{S6a}$$

$$\hat{a}^\dagger_p = \frac{1}{2}(X_p - \mathrm{i}\, Y_p) \prod_{k=1}^{p-1} Z_k, \tag{S6b}$$

where $X_p$, $Y_p$, $Z_p$ are the Pauli matrices acting on qubit $p$. In this transformation, the strings of Pauli-$Z$ matrices account for the parity of the state, as required for fermionic antisymmetry. Assuming $r > s > q > p$ without loss of generality, the qubit representation of the fermionic one-body and two-body operators is

$$F^q_p = \frac{\mathrm{i}}{2}\Big(Y_p X_q - X_p Y_q\Big) \prod_{k=p+1}^{q-1} Z_k, \tag{S7a}$$

$$\begin{aligned}F^{rs}_{pq} = \frac{\mathrm{i}}{8}\Big(&X_p X_q Y_s X_r + Y_p X_q Y_s Y_r + X_p Y_q Y_s Y_r + X_p X_q X_s Y_r \\ &- Y_p X_q X_s X_r - X_p Y_q X_s X_r - Y_p Y_q Y_s X_r - Y_p Y_q X_s Y_r\Big) \prod_{k=p+1}^{q-1} Z_k \prod_{l=r+1}^{s-1} Z_l,\end{aligned} \tag{S7b}$$

where the $F^{q\cdots}_{p\cdots}$ notation distinguishes these as the qubit versions of the second quantised operators $\hat{\kappa}^{q\cdots}_{p\cdots}$.

To prepare a wave function on a qubit register, the unitary transformations $\exp\big(t\, F^q_p\big)$ and $\exp\big(t\, F^{rs}_{pq}\big)$ need to be decomposed into elementary one- and two-qubit gates.[6] Such circuits involve applying a series of CNOT gates, known as a CNOT cascade,

that implements the parity-computing action of the Pauli-$Z$ strings in Eq. (S7). These $Z$-strings are highly non-local as they act on $\mathcal{O}(N)$ spin-orbitals. Consequently, imposing the fermionic anticommutation relations on qubit operators requires a number of CNOT gates that scales linearly with the size of the single-particle basis, dominating the CNOT cost of fermionic *ansätze*. The development of qubit-excitation operators[17,36] has been proposed to remove the $Z$-strings in Eq. (S7) and reduce the number of CNOT gates, but this formalism does not satisfy fermionic antisymmetry.

### S2.2 Operators in s-UPS ansatz

The s-UPS ansatz introduced in the main text uses an operator pool of spin-adapted one-body operators $\hat{\kappa}_p^q + \hat{\kappa}_{\bar{p}}^{\bar{q}}$ and paired two-body operators $\hat{\kappa}_{p\bar{p}}^{q\bar{q}}$. Since the one-body operators commute ($[\hat{\kappa}_p^q, \hat{\kappa}_{\bar{p}}^{\bar{q}}] = 0$ and $[F_p^q, F_{\bar{p}}^{\bar{q}}] = 0$), the exponential of the spin-adapted qubit operators can be written as $\exp\big(t(F_p^q + F_{\bar{p}}^{\bar{q}})\big) = \exp\big(tF_p^q\big)\exp\big(tF_{\bar{p}}^{\bar{q}}\big)$. We can therefore concatenate the circuits for each one-body spin-up and spin-down operator in a series and assign the same variational parameter to both, removing a degree of freedom from the parametrised *ansatz*.

Paired two-body operators are more gate-efficient compared to general two-body operators because the CNOT-overhead due to the parity computation vanishes if we define the ordering of qubits such that spin-up and spin-down orbitals which share the same spatial wave function are adjacent i.e., $\bar{p} = p + 1$ and $\bar{q} = q + 1$. Inserting these index definitions into Eq. (S7), we see that the products of $Z$-operators vanish for the qubit operators corresponding to fermionic paired two-body operators $F_{p\bar{p}}^{q\bar{q}}$, giving

$$
\begin{aligned}
F_{p\bar{p}}^{q\bar{q}} = \frac{\mathrm{i}}{8}\Big( & X_p X_{p+1} Y_q X_{q+1} + Y_p X_{p+1} Y_q Y_{q+1} + X_p Y_{p+1} Y_q Y_{q+1} + X_p X_{p+1} X_q Y_{q+1} \\
& - Y_p X_{p+1} X_q X_{q+1} - X_p Y_{p+1} X_q X_{q+1} - Y_p Y_{p+1} Y_q X_{q+1} - Y_p Y_{p+1} X_q Y_{q+1} \Big).
\end{aligned}
\tag{S8}
$$

Consequently, there is no parity-induced CNOT overhead for paired two-body fermionic operators and the number of CNOT gates required for their implementation is constant, as opposed to the $\mathcal{O}(N)$ CNOT scaling with respect to the number of spin orbitals and the excitation indices for general (unpaired) two-body operators. In fact, the operators are equivalent to the qubit excitations in Ref. 36. Removing the scaling of the CNOT count with respect to the number of spin orbitals will be especially important for larger systems since the implementation of two-qubit entangling gates is the main source of decoherence on noisy quantum hardware.

### S2.3 Circuit costs

Different circuit primitives exist for implementing fermionic operators (see Ref. 36 for a detailed discussion). The CNOT counts for our simulations (Fig. 5 in the main text) are based on the quantum circuits presented in Ref. 36 because these implementations were also used in Ref. 17, which contains the data that we compare our results against. In this approach, the number of CNOT gates required for each spin-adapted one-body fermionic operator $\exp\big(t(F_p^q + F_{\bar{p}}^{\bar{q}})\big)$ in the s-UPS ansatz is $4(p-q)+2 \geq 10$ , while paired two-body operators $\exp\big(tF_{p\bar{p}}^{q\bar{q}}\big)$ have a constant CNOT cost of 13.

## S3. Summary of the DISCO-VQE algorithm

This section summarises the implementation of the DISCO-VQE algorithm that is outlined in Fig. 1 in the main text.

### S3.1 Continuous optimisation using basin-hopping

For a given ordered set of $M$ operators $\boldsymbol{\mu}$ with the wave function

$$
|\Psi(\boldsymbol{t}, \boldsymbol{\mu})\rangle = \prod_{i=1}^{M} \mathrm{e}^{t_i \hat{\kappa}_{\mu_i}} |\Phi_0\rangle\,,
\tag{S9}
$$

the electronic energy is defined by the expectation value

$$
E(\boldsymbol{t}, \boldsymbol{\mu}) = \langle\Phi_0|\mathrm{e}^{-t_M \hat{\kappa}_{\mu_M}} \cdots \mathrm{e}^{t_1 \hat{\kappa}_{\mu_1}} \hat{H} \mathrm{e}^{t_1 \hat{\kappa}_{\mu_1}} \cdots \mathrm{e}^{t_M \hat{\kappa}_{\mu_M}} |\Phi_0\rangle\,.
\tag{S10}
$$

We use the lowest-energy restricted Hartree–Fock solution[46] to define the initial state $|\Phi_0\rangle$, although more advanced initial states could be considered. The corresponding energy landscape is highly non-linear with respect to the continuous coordinates $\boldsymbol{t}$ with the potential for several local minima. Minimisation of the continuous coordinates is performed using a customised L-BFGS[47] (limited memory Broyden,[48] Fletcher,[49] Goldfarb,[50] Shanno[51]) routine implemented in GMIN.[52] Since we consider

only real-valued operators, Hamiltonians, and coordinates, the analytic energy gradients are given by

$$\frac{\partial E(\boldsymbol{t},\boldsymbol{\mu})}{\partial t_j} = 2\left\langle \Psi(\boldsymbol{t},\boldsymbol{\mu})\right| \left( \hat{H} \left( \prod_{i=1}^{j} e^{t_i \hat{\kappa}_{\mu_i}} \right) \hat{\kappa}_{\mu_j} \left( \prod_{i=j+1}^{M} e^{t_i \hat{\kappa}_{\mu_i}} \right) \right) \left| \Phi_0 \right\rangle . \tag{S11}$$

These analytic gradients can be efficiently evaluated using the algorithm described in the supplementary information for Ref. 13.

We use the basin-hopping[29,30] procedure to systematically search for the global minimum on this continuous energy landscape with a fixed set of operators $\boldsymbol{\mu}$. Basin-hopping uses random perturbations followed by minimisation to step between local minima on the continuous energy landscape, as described in detail elsewhere [see Ref. 53]. In summary, random steps in the continuous coordinate space are taken from the current minimum, with energy $E_{\text{old}}$, and the coordinates are re-optimised to obtain a new minimum with energy $E_{\text{new}}$. A Metropolis condition is used to accept steps if $E_{\text{new}} < E_{\text{old}}$, or if $E_{\text{old}} > E_{\text{new}}$ and $\exp((E_{\text{old}} - E_{\text{new}})/T_{\text{BH}})$ is greater than a random number in the range $[0, 1]$. Here, $T_{\text{BH}}$ is a fictitious temperature that controls the magnitude of the energy increase for accepted uphill steps. This approach allows basin-hopping to systematically overcome the barriers between different minima on a continuous energy landscape. Periodic boundary conditions are used for the continuous coordinates, with the corresponding periodicity pre-computed using the eigenvalues of the (de)excitation operator matrix representations.

### S3.2 Performing discrete steps

Following a series of continuous basin-hopping steps, the lowest-energy continuous coordinates are saved and a series of discrete steps are tested. First, we consider the operator sets that can be reached by performing a cyclic permutation of the ordered set, before then considering mutations of each operator, and finally considering every possible swap between the position of two operators. The algorithm for each process is described below.

Cyclic permutations provide a way to quickly re-organise the ordered operator set without changing the relative position of certain operators. This discrete step is particularly useful in the early stages of the optimisation process where operators may be wrongly placed too close to the reference state. However, later in the optimisation we find that cyclic permutations rarely lower the energy and can have a detrimental impact on convergence. Therefore, a cyclic permutation is only accepted if it lowers the energy. These discrete steps are tested by starting from the best set of coefficients $(\boldsymbol{t}_0, \boldsymbol{\mu}_0)$ with energy $E_0$ identified in the most recent set of basin-hopping steps. For each possible cyclic permutation $j$, we permute both $\boldsymbol{t}$ and $\boldsymbol{\mu}$ and perform a single minimisation to obtain the optimised energy $E_j$. We then identify the lowest energy permutation $E_k$ and accept this discrete step if $E_k < E_0$ (Algorithm 1). If the step is accepted, then the best coordinates and ordered operator set $(\boldsymbol{t}_0, \boldsymbol{\mu}_0)$ and the energy $E_0$ are updated with the new optimised variables.

**Algorithm 1:** Procedure for testing discrete cyclic permutations.

```
Current energy, continuous coordinates, and discrete operators
E_0, t_0, μ_0

Loop over possible permutations
for j = 1, M − 1 do
  | Permute continuous coordinates and operators by j positions
  | t_j, μ_j = permute(t_0, μ_0, j)
  |
  | Minimise energy and save result
  | E_j = minimise(t_j, μ_j)
end

Find index for the lowest energy permutation
k = find_min(E_1, ..., E_{M−1})

Return best result if energy is lower than initial state
if E_k < E_0 then
  | return E_k, t_k, μ_k
else
  | return E_0, t_0, μ_0
end
```

Operator mutations are the primary mechanism for changing the type of operators in the ordered set $\boldsymbol{\mu}$ and are considered once the best cyclic permutation has been selected, with variables $(\boldsymbol{t}_0, \boldsymbol{\mu}_0)$ and energy $E_0$. The mutation of each operator is considered

individually, starting with the operator closest to the reference state (position $M$). The discrete search proceeds by testing every possible mutation of each operator $i$ with an operator $j$ selected from the pool with size $N_{\text{pool}}$. Following the mutation of an operator, a line search is performed to identify the best corresponding coordinate while the remaining coordinates are fixed. The result is then used as the initial guess for a minimisation of all the continuous coordinates, and the optimal energy is stored as $E_j$. Once all mutations for the operator $i$ have been tested, a low-energy discrete step is selected based on the criterion described in Algorithm 4 and acceptance of this step is determined using a Metropolis criterion detailed in Algorithm 5. This process is then repeated for the next operator in the ordered set. A taboo criterion is used to ensure that uphill steps do not lead to cycling between a subset of operator orderings. This algorithm is outlined in Algorithm 2.

**Algorithm 2:** Procedure for taking discrete operator mutation steps. Routines for selecting a discrete step (select_step) and testing whether to accept it (test_step) are described in Algorithms 4 and 5 respectively.

```
Current energy, continuous coordinates, and discrete operators
E_0, t_0, μ_0

Save initial energy for testing uphill steps
E_best ← E_0

Loop over operator positions, starting closest to the reference
for i = M, 1 do
    Loop over operators in the pool
    for j = 1, N_pool do
        Reset coordinates and discrete operators
        t_j ← t_0; μ_j ← μ_0

        Mutate operator at position i into operator j
        μ_j(i) ← j

        Check if new operator ordering is not taboo
        allow ← check_not_taboo(μ_j)

        if allow then
            Optimise i-th continuous coordinate using a line search
            t_j(i) ← line_search(t_j, μ_j, i)

            Minimise energy and save result
            E_j = minimise(t_j, μ_j)
        end

        Select mutation to test using fictitious temperature T_d
        k ← select_step(E_j, E_0, T_d)

        Determine whether to accept the step using fictitious temperature T_d
        accept ← test_step(E_k, E_0, E_best, T_d)

        if accept then
            Update current energy, continuous coordinates, and discrete operators
            E_0 ← E_k
            t_0 ← t_k
            μ_0 ← μ_k
        end
    end
end

Return best result
return E_0, t_0, μ_0
```

Swapping the position of two operators allows the relative ordering to be changed while retaining the overall composition of the ordered operator set. These discrete steps are considered after the operator mutations have been tested and start with the optimal

variables $(\boldsymbol{t}_0, \boldsymbol{\mu}_0)$ with energy $E_0$. Like the operator mutations, the pair swaps for each operator are considered individually, starting with the operator closest to the reference state (position $M$). The discrete search proceeds by testing every possible swap between this operator $i$ and the another $j$ in the ordered operator set. Once the operators and the corresponding continuous coordinates have been swapped, the configuration is optimised to identify the energy $E_j$. A low-energy discrete step is then selected using the algorithm described in Algorithm 4 and the acceptance of this step is determined using a Metropolis criterion detailed in Algorithm 5. This process is then repeated for the next operator in the ordered set. A taboo criterion is used to ensure that uphill steps do not lead to cycling between operator orderings. This algorithm is outlined in Algorithm 3.

**Algorithm 3:** Procedure for taking discrete operator swap steps. Routines for selecting a discrete step (select_step) and testing whether to accept it (test_step) are described in Algorithms 4 and 5 respectively.

```
Current energy, continuous coordinates, and discrete operators
E_0, t_0, μ_0

Save initial energy for testing uphill steps
E_best ← E_0

Loop over operator positions, starting closest to reference
for i = M, 1 do
    Loop over position in the ordered operator set
    for j = 1, M do
        Reset coordinates and discrete operators
        t_j ← t_0; μ_j ← μ_0

        Swap operators and coordinates at positions i and j
        μ_j(i, j) ← μ_j(j, i)
        t_j(i, j) ← t_j(j, i)

        Check if new operator ordering is not taboo
        allow ← check_not_taboo(μ_j)

        if allow then
            Minimise energy and save result
            E_j = minimise(t_j, μ_j)
        end

        Select mutation to test using fictitious temperature T_d
        k ← select_step(E_j, E_best, T_d)

        Determine whether to accept the step using fictitious temperature T_d
        accept ← test_step(E_k, E_0, E_best, T_d)

        if accept then
            Update current energy, continuous coordinates, and discrete operators
            E_0 ← E_k
            t_0 ← t_k
            μ_0 ← μ_k
        end
    end
end

Return best result
return E_0, t_0, μ_0
```

### S3.3 Taking uphill discrete steps

The discrete landscape of ordered operator sets can have many local minima, and efficient global optimisation requires uphill moves to escape these traps. Therefore, we include a further Metropolis-Hastings condition[54,55] with a second fictitious

temperature parameter $T_\mathrm{d}$ to accept uphill steps for biminima, analogous to standard basin-hopping between local minima in the continuous parameter space.[29,30] To ensure that we do not compromise the optimisation towards a given biminimum, these uphill steps are only considered when a full macro-cycle of discrete steps and continuous basin-hopping does not lower the energy and the algorithm is stuck in a biminimum. The energy after the last downhill step is recorded as $E_\mathrm{best}$.

When moving uphill, there is often a choice between many discrete steps with a similar energy. A test step is selected with a certain probability based on the energy difference relative to the lowest-energy discrete step under consideration. Specifically, if the lowest discrete step $E_\mathrm{min}$ increases the energy relative to the last downhill step (i.e. $E_\mathrm{min} > E_\mathrm{best}$), then the probability of selecting a step with energy $E_j$ is given by $\exp(-(E_j - E_\mathrm{min})/T_\mathrm{d})$. Note that $T_\mathrm{d}$ does not have to be the same as the temperature used for controlling continuous basin-hopping steps $T_\mathrm{BH}$. Any step which decreases the energy relative to the last downhill step ($E_\mathrm{min} < E_\mathrm{best}$) is always selected. This approach, summarised in Algorithm 4, avoids any artificial bias in the algorithm towards a particular nearly-degenerate step. In addition, when uphill steps are not being considered, degenerate downhill discrete steps are selected with an equal probability.

**Algorithm 4:** Procedure for selecting temperature dependent steps.

```
Energies for n discrete steps under consideration, and last downhill step
E_j, E_best

Control variable for uphill steps
uphill

Identify lowest energy after discrete steps
E_min = min_{j=1,n}(E_j)

Compute probabilities P(j) for taking step j
for j=1,n do
    if uphill or E_min > E_best then
        P(j) = exp(-(E_j - E_min)/T_d)
    else
        if E_j = E_min then
            P(j) = 1
        else
            P(j) = 0
        end
    end
end

Normalise the probabilities
P(j) = P(j) / sum_{j=1,n}(P(k))

Randomly select a discrete step using computed probabilities
k = random_select(P(1 : n))

Return selected step index
return k
```

Once a step with energy $E_k$ has been selected using Algorithm 4, it is either accepted or rejected based on a a Metropolis criteria using the same fictitious temperature $T_\mathrm{d}$. When uphill steps are not being considered ($uphill$ = False), discrete steps are only accepted if $E_k < E_0$. When uphill steps are being considered ($uphill$ = True), a discrete step with energy $E_k$ is accepted if it lowers the energy relative to the last step, $E_k < E_0$, or with probability $\exp(-(E_k - E_0)/T_\mathrm{d})$ if $E_k > E_0$. If any discrete step lowers the energy below the last downhill step, $E_k < E_\mathrm{best}$, then no further uphill steps are considered in the current macro-cycle (i.e. $uphill \rightarrow$ False). This condition ensures that we do not take any more uphill steps than are needed to escape a biminimum. The algorithm for accepting or rejecting proposed discrete steps is detailed in Algorithm 5.

**Algorithm 5:** Procedure for testing temperature-dependent steps.

Energies of proposed step $k$, last step, and last downhill step
$E_k, E_0, E_{\text{best}}$

Control variable for uphill steps
*uphill*

Turn off uphill steps if energy goes below last downhill step
**if** $E_k < E_{best}$ **then**
  *uphill* $\leftarrow$ False
**end**

Compute probability $P$ for accepting step
**if** $E_k < E_0$ **then**
  Always accept a downhill step
  $P \leftarrow 1$
**else**
  Otherwise accept based on Metropolis criterion
  **if** *uphill* **then**
    $P = \exp(-(E_k - E_0)/T_{\text{d}})$
  **else**
    $P = 0$
  **end**
**end**

Test if step is accepted using a random number in range $[0, 1]$
*accept* $= P > \text{random}(0, 1)$

**return** *accept*

We also employ the basin-hopping parallel tempering (BHPT) scheme[56] to improve efficiency. Multiple generalised basin-hopping runs, comprising the continuous and discrete optimisation steps, are performed in parallel using different temperature parameters for accepting moves between biminima, with exchange between replicas analogous to the parallel tempering formalism.[57] The different temperatures apply to the Metropolis criteria used in both the continuous basin-hopping and discrete uphill steps (i.e., $T_{\text{BH}} = T_{\text{d}}$). In this approach, the high-temperature replicas can efficiently move over high barriers on the energy landscape while low-temperature replicas fine-tune the optimisation in each basin of attraction. Finally, we employ a taboo criterion to encourage the discrete search to climb uphill out of biminima and prevent cycling between a local neighbourhood of ordered operator sets. In this approach, a taboo is placed on ordered sets of operators that prevent a given configuration from being revisited within a certain number of discrete steps $N_{\text{t}}$.

### S3.4 Summary of hyperparameters

In addition to the standard basin-hopping methodology, the DISCO-VQE algorithm introduces the following hyperparameters:

- **Number of Basin-Hopping steps ($N_{\text{BH}}$)**
  The number of basin-hopping steps performed on each macrocycle DISCO-VQE;
- **Taboo delay ($N_{\text{t}}$)**
  A particular ordered set of operators cannot be revisited within $N_{\text{t}}$ discrete steps;
- **Discrete temperature ($T_{\text{d}}$)**
  The fictitious temperature associated with selecting and accepting discrete uphill steps.

Preliminary numerical studies identified suitable values as $N_{\text{BH}} = 100$, $N_{\text{t}} = 20$, and $T_{\text{d}} = 0.0001$–$0.01\,\text{E}_{\text{h}}$.

### S3.5 Computational implementation

We have implemented DISCO-VQE in the GMIN program,[52] developed by some of us for finding global minima on continuous energy landscapes. We use PySCF[58] to generate reference Hartree–Fock solutions and the corresponding one- and two-electron Hamiltonian integrals. We then use OpenFermion[59] to generate Hilbert-space matrix representations of the Hamiltonian operator and the anti-Hermitian spin-adapted one-body and paired two-body (de)excitation operators. These matrices provide the input for DISCO-VQE calculations in GMIN, where all subsequent computations are performed. All calculations are performed with the restricted Hartree–Fock[46] reference as the initial state, corresponding to an empty set of unitary operators and $\boldsymbol{t} = \mathbf{0}$.

# S4. Linear and tetrahedral $H_4$ (STO-3G)

## S4.1 Computational Details

The same calculation setup was used for the convergence with respect to the number of operators and the full DISCO-VQE ground-state binding curves in both linear and tetrahedral $H_4$:

- 8 BHPT replicas at temperatures distributed exponentially from $0.0001$ to $0.01\,\mathrm{E_h}$. Replica exchange considered after every 10 continuous basin–hopping steps. Same fictitious temperature for basin–hopping steps and discrete uphill steps ($T_{\mathrm{BH}} = T_{\mathrm{d}}$);
- Maximum continuous step size of $0.5$, updated dynamically to give an average $50\,\%$ acceptance;
- Total of $100\,000$ basin–hopping steps;
- $N_{\mathrm{BH}} = 100$ basin–hopping steps for each DISCO-VQE macrocycle;
- Taboo delay of $N_{\mathrm{t}} = 20$.

For the linear $H_4$ binding curves computed using twenty fixed random orderings of 13 operators and the the best operator ordering identified at $R(\mathrm{H{-}H}) = 0.9\,\text{Å}$, the optimisation was only performed for the continuous coordinates using the BHPT approach. The following input parameters were used:

- 8 BHPT replicas at temperatures distributed exponentially from $0.0001$ to $0.01\,\mathrm{E_h}$. Replica exchange considered after every 10 continuous basin–hopping steps;
- Maximum continuous step size of $0.5$, updated dynamically to give an average $50\,\%$ acceptance;
- Total of $100\,000$ basin–hopping steps.

## S4.2 Binding curve using a fixed *ansatz*

The optimal operator ordering identified with thirteen operators at a bond length of $0.90\,\text{Å}$ was used to define a fixed *ansatz* that was tested across the full binding curve. BHPT calculations were performed to identify the optimal continuous coordinates at each bond length. This fixed *ansatz* gives exact energies at the majority of bond lengths considered and has a maximum error of $0.379\,\mu\mathrm{E_h}$ (Fig. S2). The accuracy of this *ansatz* demonstrates the transferability of optimal DISCO-VQE wave functions across different geometries.

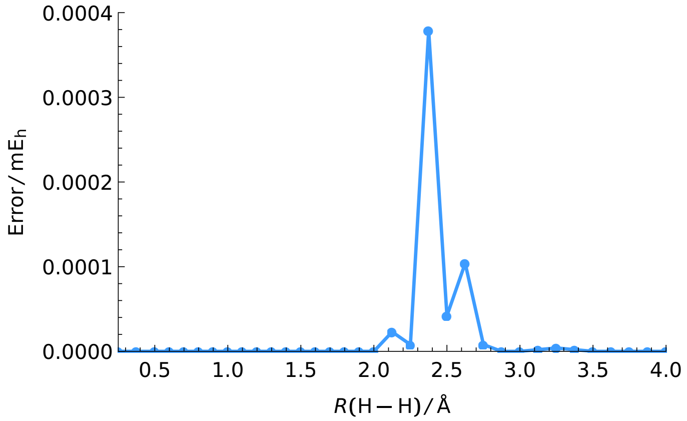


FIG. S2: Error for linear $H_4$ (STO-3G) using the optimal DISCO-VQE(13) *ansatz* identified at $R(\mathrm{H{-}H}) = 0.90\,\text{Å}$.

## S4.3 Comparison of DISCO-VQE and ADAPT-VQE binding curves

The energetic error for truncated DISCO-VQE approximations is compared to ADAPT-VQE across the full linear $H_4$ (STO-3G) binding curve in Fig. S3. ADAPT-VQE calculations, implemented in GMIN, were performed with the same operator pool with no restriction on the number of operators and were considered converged when the energy no longer changed on each iteration. DISCO-VQE calculations with six operators give more accurate energies than ADAPT-VQE, giving a non-parallelity error (NPE) of $12.02\,\mathrm{mE_h}$ compared to $33.05\,\mathrm{mE_h}$ for ADAPT-VQE. Ten operators is sufficient for DISCO-VQE to give a chemically accurate binding curve with NPE $= 0.29\,\mathrm{mE_h}$.

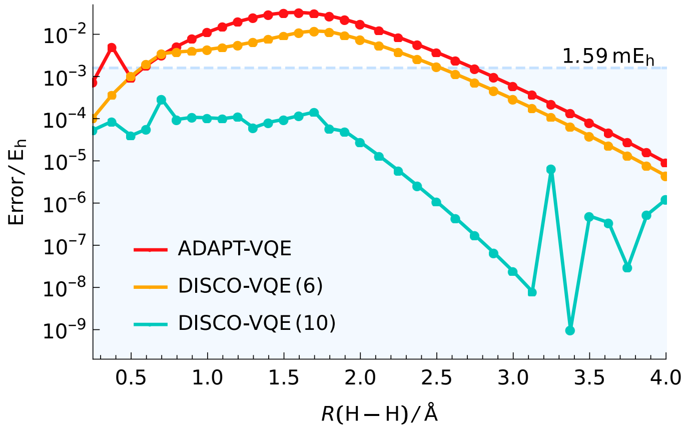


FIG. S3: Comparison of the energy error for linear $H_4$ (STO-3G) using truncated DISCO-VQE approximations and ADAPT-VQE. The NPE for ADAPT-VQE, DISCO-VQE(6) and DISCO-VQE(10) are $33.05$, $12.02$, and $0.29\,\mathrm{mE_h}$ respectively.

## S5. Linear $H_6$ binding curve (STO-3G)

### S5.1 Computational Details

DISCO-VQE calculations for the linear $H_6$ binding curve employed the following parameters:

- 8 BHPT replicas at temperatures distributed exponentially from $0.0001$ to $0.01\,\mathrm{E_h}$. Replica exchange considered after every 10 continuous basin–hopping steps. Same fictitious temperature for basin–hopping steps and discrete uphill steps ($T_{\mathrm{BH}} = T_{\mathrm{d}}$);
- Maximum continuous step size of $0.5$, updated dynamically to give an average $50\,\%$ acceptance;
- $N_{\mathrm{BH}} = 100$ basin–hopping steps for each DISCO-VQE macrocycle;
- Taboo delay of $N_{\mathrm{t}} = 20$.

To improve the likelihood of finding the global minimum, calculations for $R(\mathrm{H{-}H}) \leq 1.2\,\text{Å}$ with 10, 20, or 30 operators were performed with $40\,000$ basin-hopping steps. Calculations for $R(\mathrm{H{-}H}) > 1.2\,\text{Å}$ with 10, 20, or 30 operators were performed with $20\,000$ basin-hopping steps, which reliably obtained the global minimum. $20,000$ basin-hopping steps were used for all calculations with 40 operators, regardless of the bond length.

ADAPT-VQE calculations are performed up to $1000$ operators to remove the effect of choosing a gradient-based convergence threshold.

## S6. Symmetric $H_2O$ binding curve (STO-3G)

### S6.1 Computational Details

The number of operators in the s-UPS wave function was fixed to the size of the operator pool, 42. DISCO-VQE calculations for the $H_2O$ symmetric stretch employed the following parameters:

- 8 BHPT replicas at temperatures distributed exponentially from $0.0001$ to $0.01\,\mathrm{E_h}$. Replica exchange considered after every 10 continuous basin–hopping steps. Same fictitious temperature for basin–hopping steps and discrete uphill steps ($T_{\mathrm{BH}} = T_{\mathrm{d}}$);
- Maximum continuous step size of $0.5$, updated dynamically to give an average $50\,\%$ acceptance;
- Total of $20\,000$ basin–hopping steps;
- $N_{\mathrm{BH}} = 100$ basin–hopping steps for each DISCO-VQE macrocycle;
- Taboo delay of $N_{\mathrm{t}} = 20$.

ADAPT-VQE calculations are performed up to $1000$ operators to remove the effect of choosing a gradient-based convergence threshold.

## S7. $N_2$ binding curve (STO-3G)

### S7.1 Computational Details

The number of operators in the s-UPS wave function was fixed to the size of the operator pool (30) and the four lowest molecular orbitals in the STO-3G were frozen. DISCO-VQE calculations for the $N_2$ binding curve employed the following parameters:

- 8 BHPT replicas at temperatures distributed exponentially from $0.0001$ to $0.01\,\mathrm{E_h}$. Replica exchange considered after every 10 continuous basin–hopping steps. Same fictitious temperature for basin–hopping steps and discrete uphill steps ($T_{\mathrm{BH}} = T_{\mathrm{d}}$);
- Maximum continuous step size of $0.5$, updated dynamically to give an average $50\,\%$ acceptance;
- Total of $20\,000$ basin–hopping steps;
- $N_{\mathrm{BH}} = 100$ basin–hopping steps for each DISCO-VQE macrocycle;
- Taboo delay of $N_{\mathrm{t}} = 20$.

### S7.2 Comparison of binding curve accuracy

Table S1 compares the mean-average error for related fermionic *ansatz* across the $N_2$ binding curve with the number of variational parameters in the wave function. The un-Trotterised $k$-UpCCGSD *ansatz*[24] requires 180 variational parameters ($k = 4$) to obtain a better mean-average error (MAE) than DISCO-VQE and 135 parameters ($k = 3$) to get a more accurate NPE. ADAPT-VQE calculations using the same operator pool do not give a qualitatively correct binding curve, giving a large MAE and NPE. Depending on the bond length, ADAPT-VQE calculations converge with between 10 to 100 operators, after which adding more operators leaves the energy unchanged.

TABLE S1: Comparison of mean-average error (MAE) and non-parallelity error (NPE) of related fermionic *ansatz* for the $N_2$ (STO-3G) binding curve. The un-Trotterised $k$-UpCCGSD results are taken from Ref. 24.

| Method | # Parameters | MAE $/\mathrm{mE_h}$ | NPE $/\mathrm{mE_h}$ |
|---|---|---|---|
| ADAPT-VQE | 10–100 | 87.88 | 242.55 |
| DISCO-VQE | 30 | 0.77 | 5.08 |
| 1-UpCCGSD | 45 | 43.16 | 41.09 |
| 2-UpCCGSD | 90 | 13.16 | 8.85 |
| 3-UpCCGSD | 135 | 2.81 | 2.45 |
| 4-UpCCGSD | 180 | 0.60 | 1.51 |
| 5-UpCCGSD | 225 | 0.31 | 0.77 |
| 6-UpCCGSD | 270 | 0.15 | 0.36 |

## S8. Two-dimensional Hubbard lattice

DISCO-VQE calculations on the $4 \times 2$ Hubbard lattice employed periodic boundary conditions along the long axis and open boundary conditions along the short axis. Since the 4900-dimensional Hilbert space is computationally expensive for BHPT, we perform DISCO-VQE using a dynamic temperature update and divide the discrete step search over parallel processes. In particular, after each set of 50 uphill discrete steps, the corresponding temperature $T_{\mathrm{d}}$ is either increased or decreased to keep the average acceptance ratio close to $50\,\%$. This temperature for discrete uphill steps is not necessarily the same as the temperature $T_{\mathrm{BH}}$ for the continuous Metropolis criteria used in the basin-hopping steps. The input parameters for these calculations are:

- Maximum continuous step size of $0.5$, updated dynamically to give an average $50\,\%$ acceptance;
- Temperature for continuous basin-hopping steps $T_{\mathrm{BH}} = 0.001\,t$;
- Initial temperature for uphill discrete steps $T_{\mathrm{d}} = 0.01\,t$, updated dynamically to give $50\,\%$ acceptance;
- $N_{\mathrm{BH}} = 100$ basin–hopping steps for each DISCO-VQE macrocycle;
- Total of $5\,000$ basin–hopping steps;
- Taboo delay of $N_{\mathrm{t}} = 20$.

Corresponding ADAPT-VQE simulations used a convergence threshold corresponding to a discrete gradient root-mean-square threshold of $10^{-4}\,t$.

## S9. References and Notes

[1] B. Bauer, S. Bravyi, M. Motta, G. K.-L. Chan, Quantum Algorithms for Quantum Chemistry and Quantum Materials Science, *Chem. Rev.* **120**, 12685 (2020).
[2] A. Aspuru-Guzik, A. D. Dutoi, P. J. Love, M. Head-Gordon, Simulated Quantum Computation of Molecular Energies, *Science* **309**, 1704 (2005).
[3] S. McArdle, S. Endo, A. Aspuru-Guzik, S. C. Benjamin, X. Yuan, Quantum computational chemistry, *Reviews of Modern Physics* **92**, 15003 (2020).
[4] A. Peruzzo, *et al.*, A variational eigenvalues solver on a photonic quantum processor, *Nat. Comm.* **5**, 4213 (2014).
[5] A. Kandala, *et al.*, Hardware-efficient variational quantum eigensolver for small molecules and quantum magnets, *Nature* **549**, 242 (2017).

[6]A. Anand, *et al.*, A quantum computing view on unitary coupled cluster theory, *Chem. Soc. Rev.* **51**, 1659 (2022).
[7]T. Helgaker, P. Jørgensen, J. Olsen, *Molecular Electronic-Structure Theory* (John Wiley & Sons, 2000).
[8]R. J. Bartlett, M. Musiał, Coupled-cluster theory in quantum chemistry, *Rev. Mod. Phys.* **79**, 291 (2007).
[9]F. A. Evangelista, G. K.-L. Chan, G. E. Scuseria, Exact parameterization of fermionic functions via unitary coupled cluster theory, *J. Chem. Phys.* **151**, 244122 (2019).
[10]A. F. Izmaylov, M. Díaz-Tinoco, R. A. Lang, On the order problem in construction of unitary operators for the variational quantum eigensolver, *Phys. Chem. Chem. Phys.* **22**, 12980 (2020).
[11]H. R. Grimsley, D. Claudino, S. E. Economou, E. Barnes, N. J. Mayhall, Is the Trotterized UCCSD Ansatz Chemically Well-Defined?, *J. Chem. Theory Comput.* **16**, 1 (2020).
[12]T. Tsuchimochi, Y. Mori, S. L. Ten-no, Spin-projection for quantum computation: A low-depth approach to strong correlation, *Phys. Rev. Research* **2**, 043142 (2020).
[13]H. R. Grimsley, S. E. Economou, E. Barnes, N. J. Mayhall, An adaptive variational algorithm for exact molecular simulations on a quantum computer, *Nat. Comm.* **10**, 3007 (2019).
[14]H. L. Tang, *et al.*, Qubit-ADAPT-VQE: An Adaptive Algorithm for Constructing Hardware-Efficient Ansätze on a Quantum Processor, *PRX Quantum* **2**, 020310 (2021).
[15]H. H. S. Chan, N. Fitzpatrick, J. Segarra-Martí, M. J. Bearpark, D. P. Tew, Molecular excited state calculations with adaptive wavefunctions on a quantum eigensolver emulation: reducing circuit depth and separating spin states, *Phys. Chem. Chem. Phys.* **23**, 26438 (2021).
[16]T. Tsuchimochi, M. Taii, T. Nishimaki, S. L. Ten-no, Adaptive construction of shallower quantum circuits with quantum spin projection for fermionic systems arxiv:2205.07097 (2022).
[17]Y. S. Yordanov, V. Armaos, C. H. W. Barnes, D. R. M. Arvidsson-Shukur, Qubit-excitation-based adaptive variational quantum eigensolver, *Commun. Phys.* **4**, 228 (2021).
[18]V. O. Shkolnikov, N. J. Mayhall, S. E. Economou, E. Barnes, Avoiding symmetry roadblocks and minimizing the measurement overhead of adaptive variational quantum eigensolvers arxiv:2109.05340 (2021).
[19]N. C. Rubin, J. Lee, R. Babbush, Compressing Many-Body Fermion Operators Under Unitary Constraints (2021).
[20]P. Jordan, E. Wigner, Über das Paulische Äquivalenzverbot, *Z. Phys.* **47**, 631 (1928).
[21]S. B. Bravyi, A. Y. Kitaev, Fermionic Quantum Computation, *Ann. Phys.* **298**, 210 (2002).
[22]R. Gilmore, *Lie Groups, Physics, and Geometry: An Introduction for Physicists, Engineers, and Chemists* (Dover Publications Inc., 2008), first edn.
[23]B. C. Hall, *Lie Groups, Lie Algebras, and Representations* (Springer Chem, 2015).
[24]J. Lee, W. J. Huggins, M. Head-Gordon, K. B. Whaley, Generalized Unitary Coupled Cluster Wave functions for Quantum Computation, *J. Chem. Theory Comput.* **15**, 311 (2019).
[25]H. R. Grimsley, G. S. Barron, E. Barnes, S. E. Economou, N. J. Mayhall, ADAPT-VQE is insensitive to rough parameter landscapes and barren plateaus arxiv:2204.07179 (2022).
[26]D. Schebarchov, D. J. Wales, Communication: A new paradigm for structure prediction in multicomponent systems, *J. Chem. Phys.* **139**, 221101 (2013).
[27]D. Schebarchov, D. J. Wales, Structure Prediction for Multicomponent Materials Using Biminima, *Phys. Rev. Lett.* **113**, 156102 (2014).
[28]K. Röder, D. J. Wales, Mutational Basin-Hopping: Combined Structure and Sequence Optimization for Biomolecules, *J. Phys. Chem. Lett.* **9**, 6169 (2018).
[29]Z. Li, H. A. Scheraga, Monte carlo-minimization approach to the multiple-minima problem in protein folding, *PNAS* **84**, 6611 (1987).
[30]D. J. Wales, J. P. K. Doye, Global Optimization by Basin-Hopping and the Lowest Energy Structures of Lennard-Jones Clusters Containing up to 110 Atoms, *J. Phys. Chem. A* **101**, 5111 (1997).
[31]W. J. Hehre, R. F. Stewart, J. A. Pople, Self-Consistent Molecular-Orbital Methods. I. Use of Gaussian Expansions of Slater-Type Atomic Orbitals, *J. Chem. Phys.* **51**, 2657 (1969).
[32]Y. Matsuzawa, Y. Kurashige, Jastrow-type Decomposition in Quantum Chemistry for Low-Depth Quantum Circuits, *J. Chem. Theory Comput.* **16**, 944 (2020).
[33]The non-parallelity error is defined as the difference between the maximum and minimum error along a binding curve.
[34]M. D. Sapova, A. K. Fedorov, Variational quantum eigensolver techniques for simulating carbon monoxide oxidation arxiv:2108.111.67 (2021).
[35]S. Sim, J. Romero, J. F. Gonthier, A. A. Kunitsa, Adaptive pruning-based optimization of parametrized quantum circuits, *Quantum Sci. Technol.* **6**, 025019 (2021).
[36]Y. S. Yordanov, D. R. M. Arvidsson-Shukur, C. H. W. Barnes, Efficient quantum circuits for quantum computational chemistry, *Phys. Rev. A* **102**, 062612 (2020).
[37]J. P. F. LeBlanc, *et al.*, Solutions of the Two-Dimensional Hubbard Model: Benchmarks and Results from a Wide Range of Numerical Algorithms, *Phys. Rev. X* **5**, 041041 (2015).
[38]J. Stokes, J. Izaac, N. Killoran, G. Carleo, Quantum natural gradient, *Quantum* **4**, 269 (2020).
[39]B. Koczor, S. C. Benjamin, Quantum analytic descent, *Phys. Rev. Research* **4**, 023017 (2022).
[40]A. G. Rattew, S. Hu, M. Pistoia, R. Chen, S. Wood, A Domain-agnostic, Noise-resistant, Hardware-efficient, Evolutional Variational Quantum Eigensolver arXiv:1910.09694 (2019).
[41]D. Chivilikhin, *et al.*, MoG-VQE: Multiobjective genetic variational quantum eigensolver arxiv:2007.04424 (2020).
[42]S.-X. Zhang, C.-Y. Hsieh, S. Zhang, H. Yao, Differentiable Quantum Architecture Search arxiv:2010.08561 (2021).
[43]M. O. E. Grant, M. Benedetti, Structure optimization for parameterized quantum circuits, *Quantum* **5**, 391 (2021).
[44]A. Anand, M. Degroote, A. Aspuru-Guzik, Natural evolutionary strategies for variational quantum computation, *Mach. Learn.: Sci. Technol.* **2**, 045012 (2021).
[45]I. Shavitt, R. Bartlett, *Many-Body Methods in Chemistry and Physics* (Cambridge University Press, 2009).
[46]A. Szabo, N. S. Ostlund, *Modern Quantum Chemistry* (Dover Publications Inc., 1989).
[47]J. Nocedal, Updating quasi-Newton matrices with limited storage, *Math. Comp.* **35**, 773 (1980).
[48]C. G. Broyden, The Convergence of a Class of Double-rank Minimization Algorithms 1. General Considerations, *IMA J. Appl. Math.* **6**, 76 (1970).
[49]R. Fletcher, A new approach to variable metric algorithms, *Comput. J.* **13**, 317 (1970).
[50]D. Goldfarb, A family of variable-metric methods derived by variational means, *Math. Comp.* **24**, 23 (1970).
[51]D. F. Shanno, Conditioning of quasi-Newton methods for function minimization, *Math. Comp.* **24**, 647 (1970).
[52]GMIN: A program for finding global minima and calculating thermodynamic properties, http://www-wales.ch.cam.ac.uk/software.html.
[53]D. J. Wales, *Energy Landscapes: Applications to Clusters, Biomolecules and Glasses* (Cambridge University Press, Cambridge, 2004).
[54]N. Metropolis, A. W. Rosebluth, M. N. Rosenbluth, A. H. Teller, E. Teller, Equation of State Calculations by Fast Computing Machines, *J. Chem. Phys.* **21**, 1087 (1953).
[55]W. K. Hastings, Monte Carlo sampling methods using Markov chains and their applications, *Biometrika* **57**, 97 (1970).
[56]B. Strodel, J. W. L. Lee, C. S. Whittleston, D. J. Wales, Transmembrane structures for alzheimer's a$\beta$1-42 oligomers, *J. Am. Chem. Soc.* **132**, 13300 (2010).

[57]R. H. Swendsen, J.-S. Wang, Replica Monte Carlo Simulation of Spin-Glasses, *Phys. Rev. Lett.* **57**, 2607 (1986).
[58]Q. Sun, *et al.*, Recent developments in the PySCF program package, *J. Chem. Phys.* **153**, 024109 (2020).
[59]J. R. McClean, *et al.*, OpenFermion: the electronic structure package for quantum computers, *Quantum Sci. Technol.* **5**, 034014 (2020).
